# Supplementary material for: Bayesianize Fuzziness in the Statistical Analysis of Fuzzy Data
Source: arXiv:2501.18974 source file (2025-04-28)
Supplement: Supplementary file 1 [file supplementary_materials.pdf]

# Bayesianize Fuzziness in the Statistical Analysis of Fuzzy Data

Antonio Calcagni\*, Przemysław Grzegorzewski, Maciej Romaniuk

## Supplementary Materials

This supplementary materials contain extended graphical results for the approximation problem of the posterior density function  $\pi(y|\boldsymbol{\theta}_y, \mathbf{D})$  described in Section 5 of the main article.

---

\*Corresponding author: antonio.calcagni@unipd.it

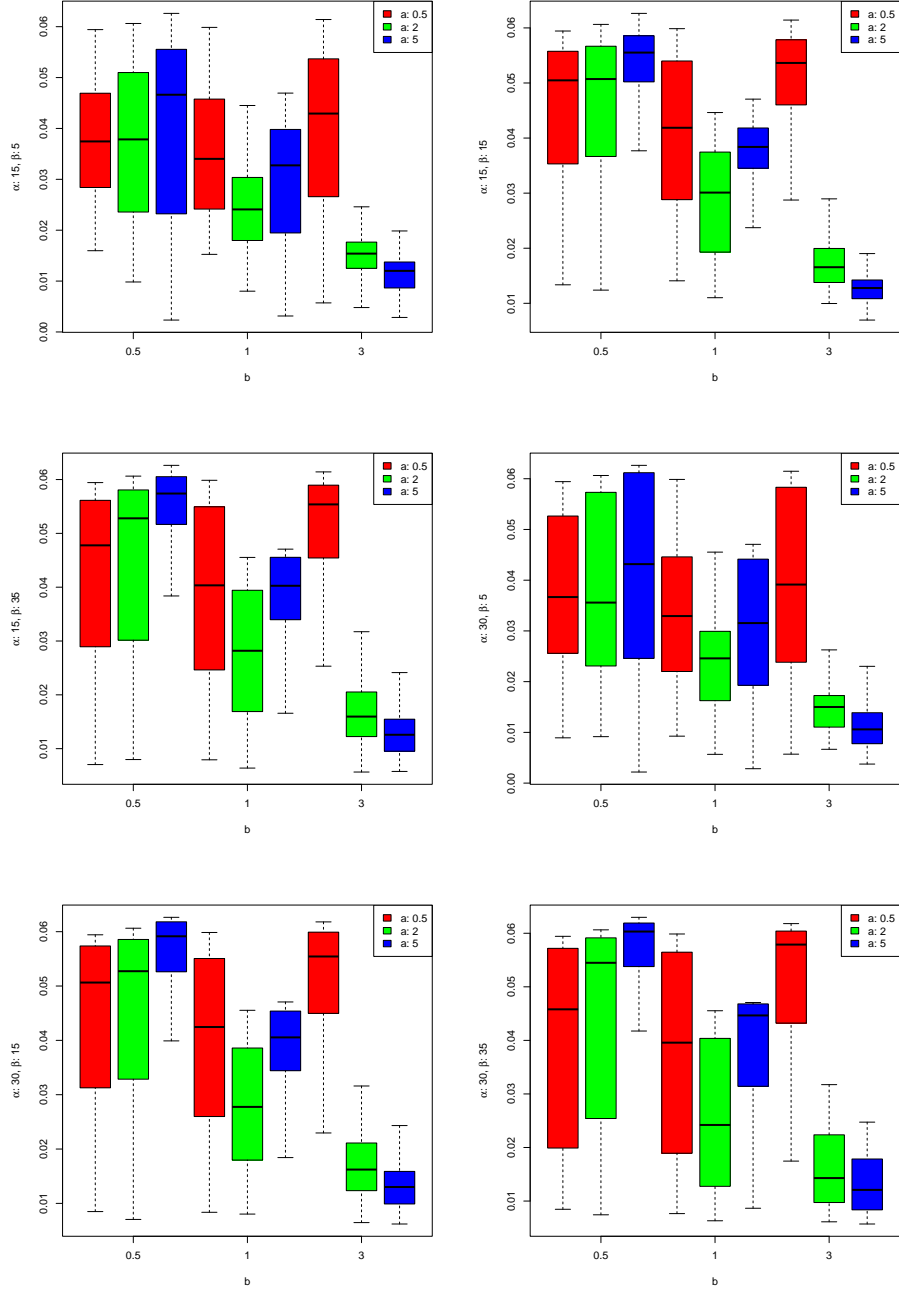

Figure S.1: Boxplots for the estimated total variation (TV) distance in the DA analysis for  $\mathcal{B}(a, b)$ .

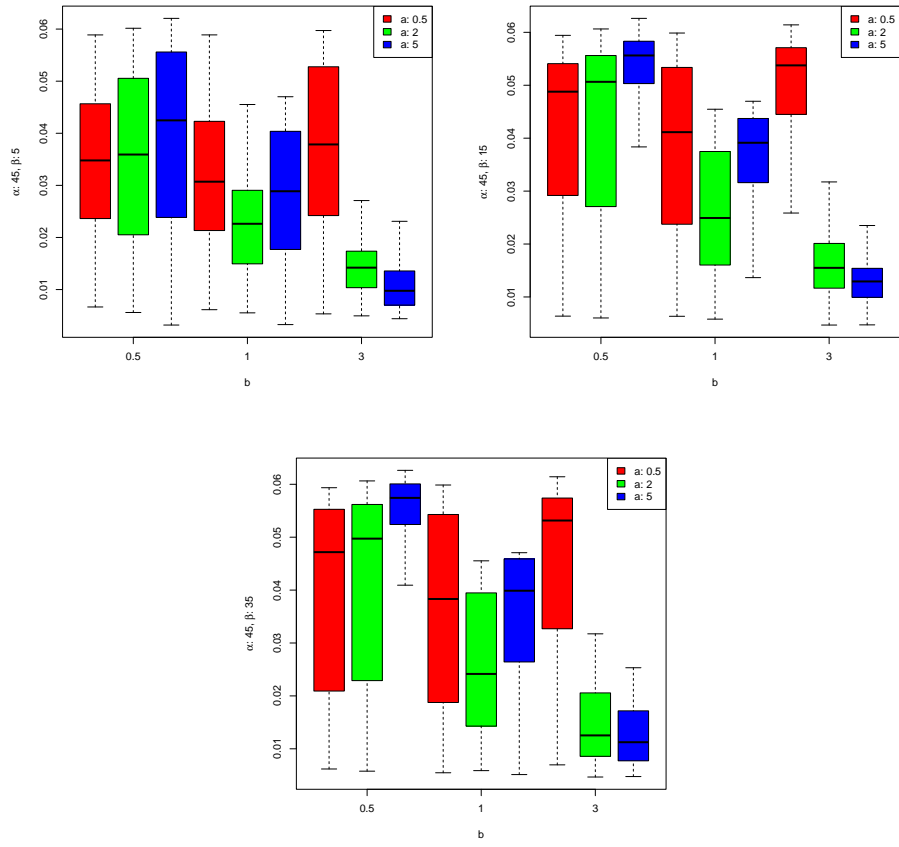

Figure S.2: Boxplots for the estimated total variation (TV) distance in the DA analysis for  $\mathcal{B}(a, b)$  (continuation).

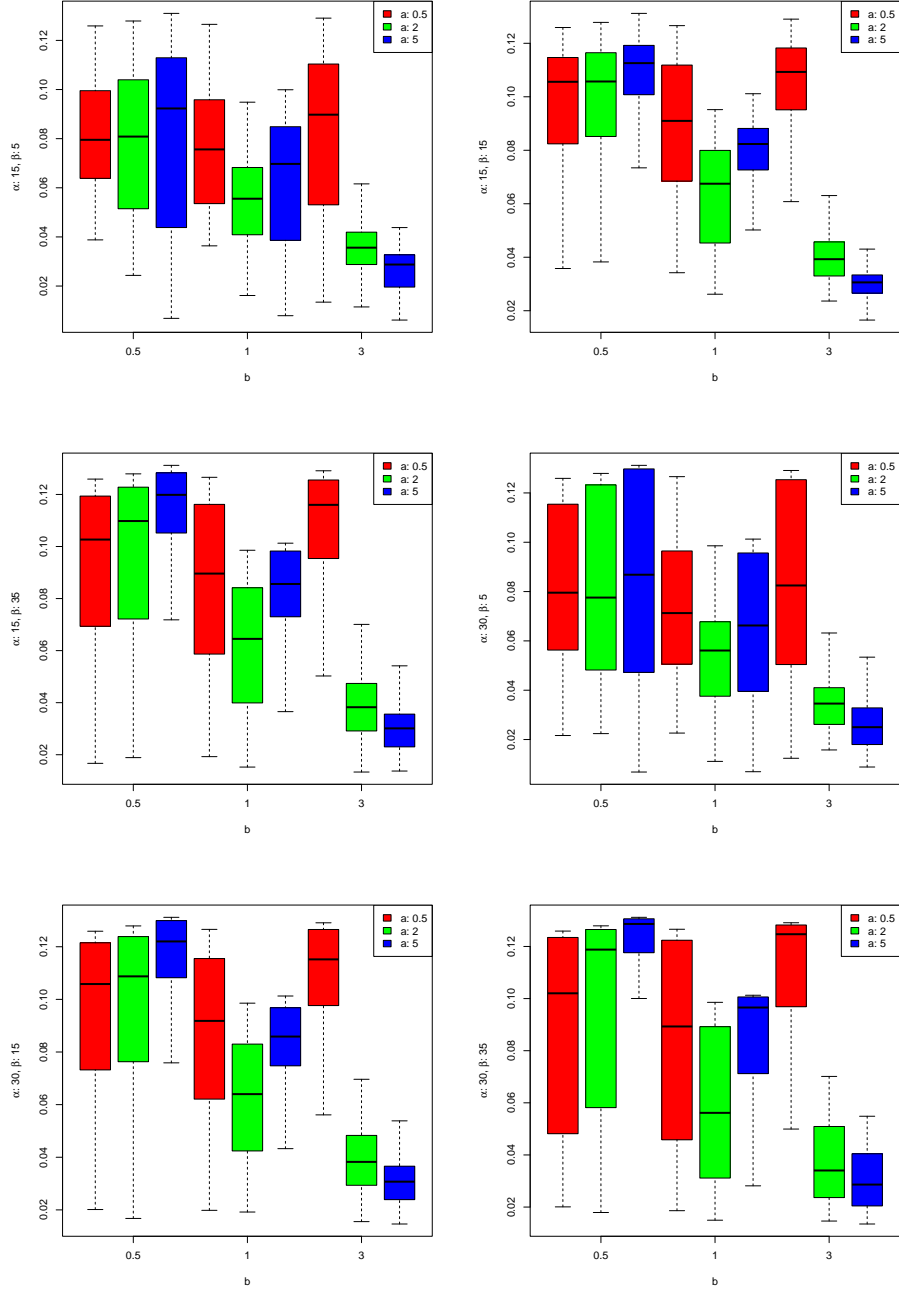

Figure S.3: Boxplots for the estimated Hellinger distance (HD) in the DA analysis for  $\mathcal{B}(a, b)$ .

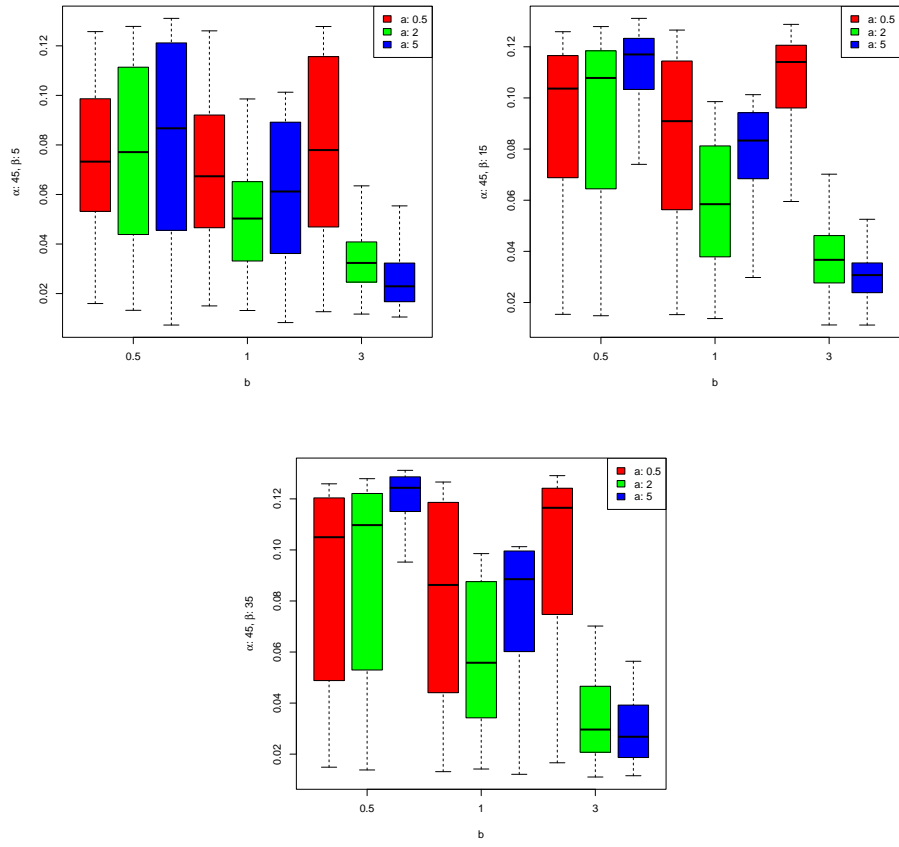

Figure S.4: Boxplots for the estimated Hellinger distance (HD) in the DA analysis for  $\mathcal{B}(a, b)$  (continuation).

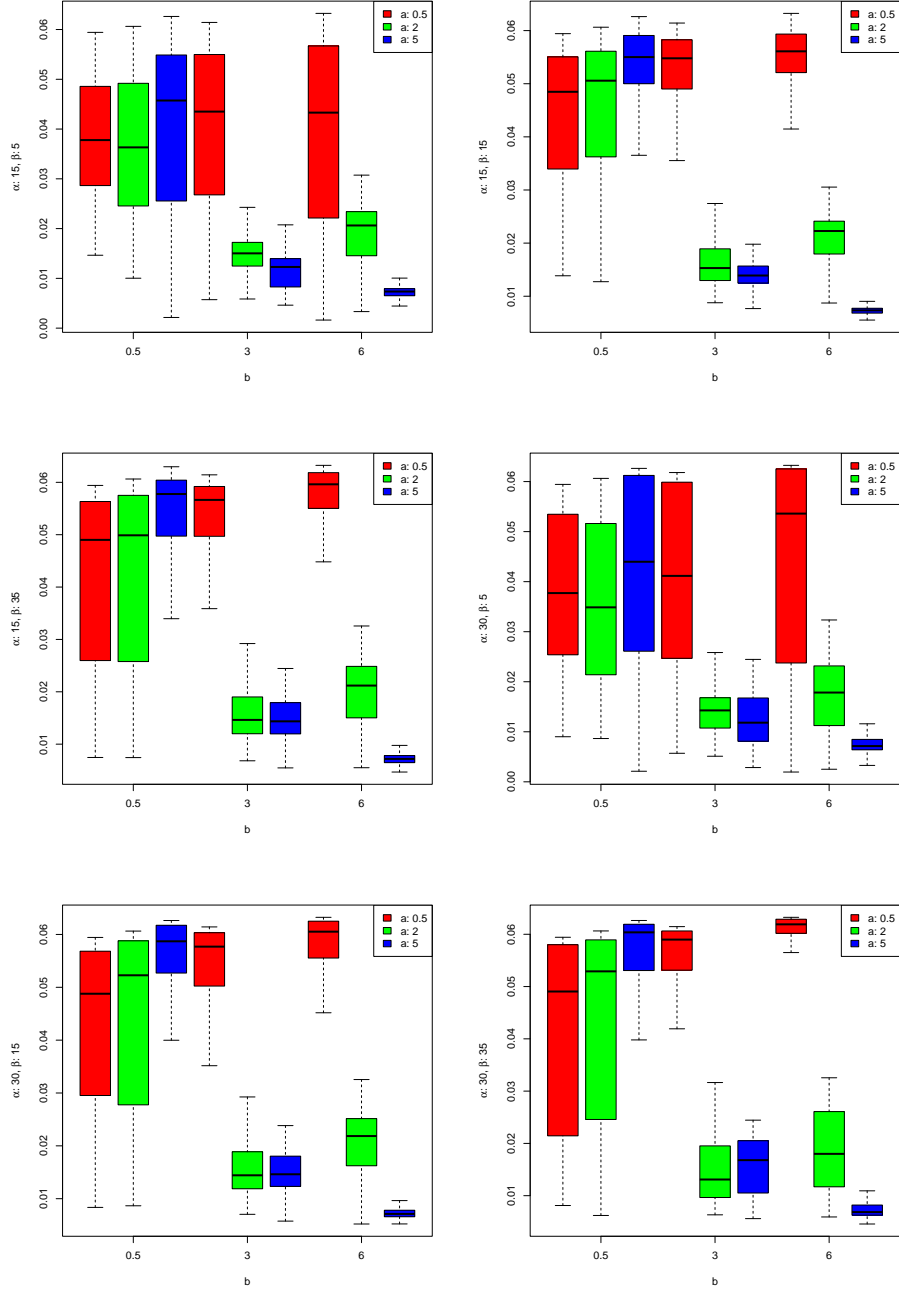

Figure S.5: Boxplots for the estimated total variation (TV) distance in the DA analysis for  $\mathcal{K}(a, b)$ .

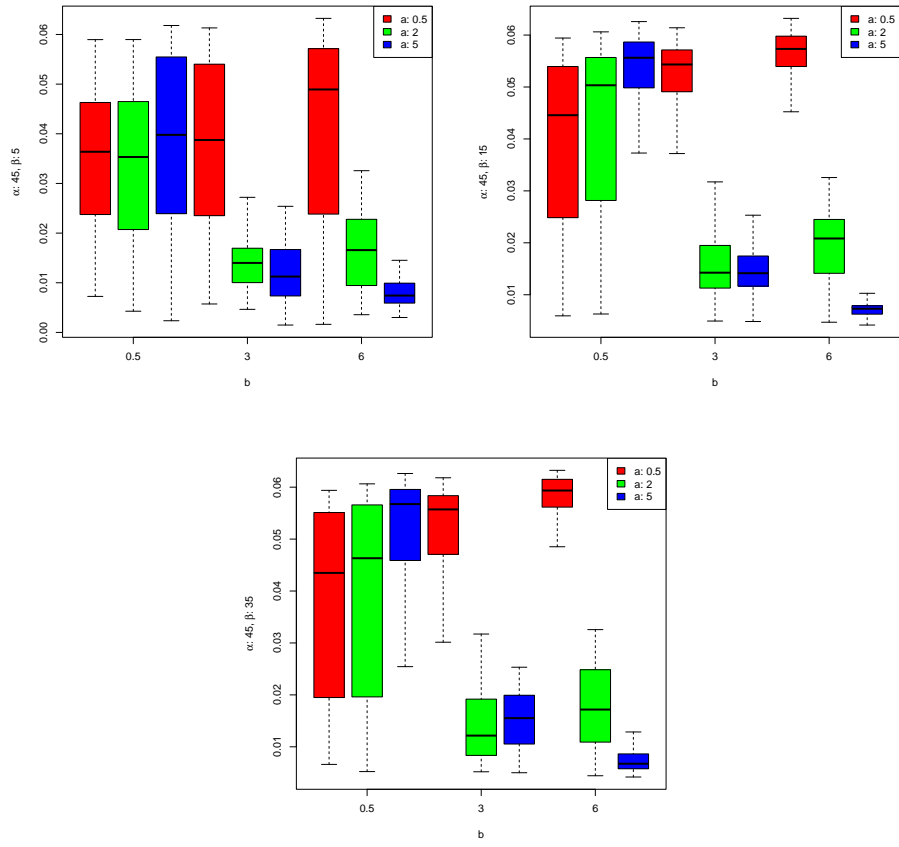

Figure S.6: Boxplots for the estimated total variation (TV) distance in the DA analysis for  $\mathcal{K}(a, b)$  (continuation).

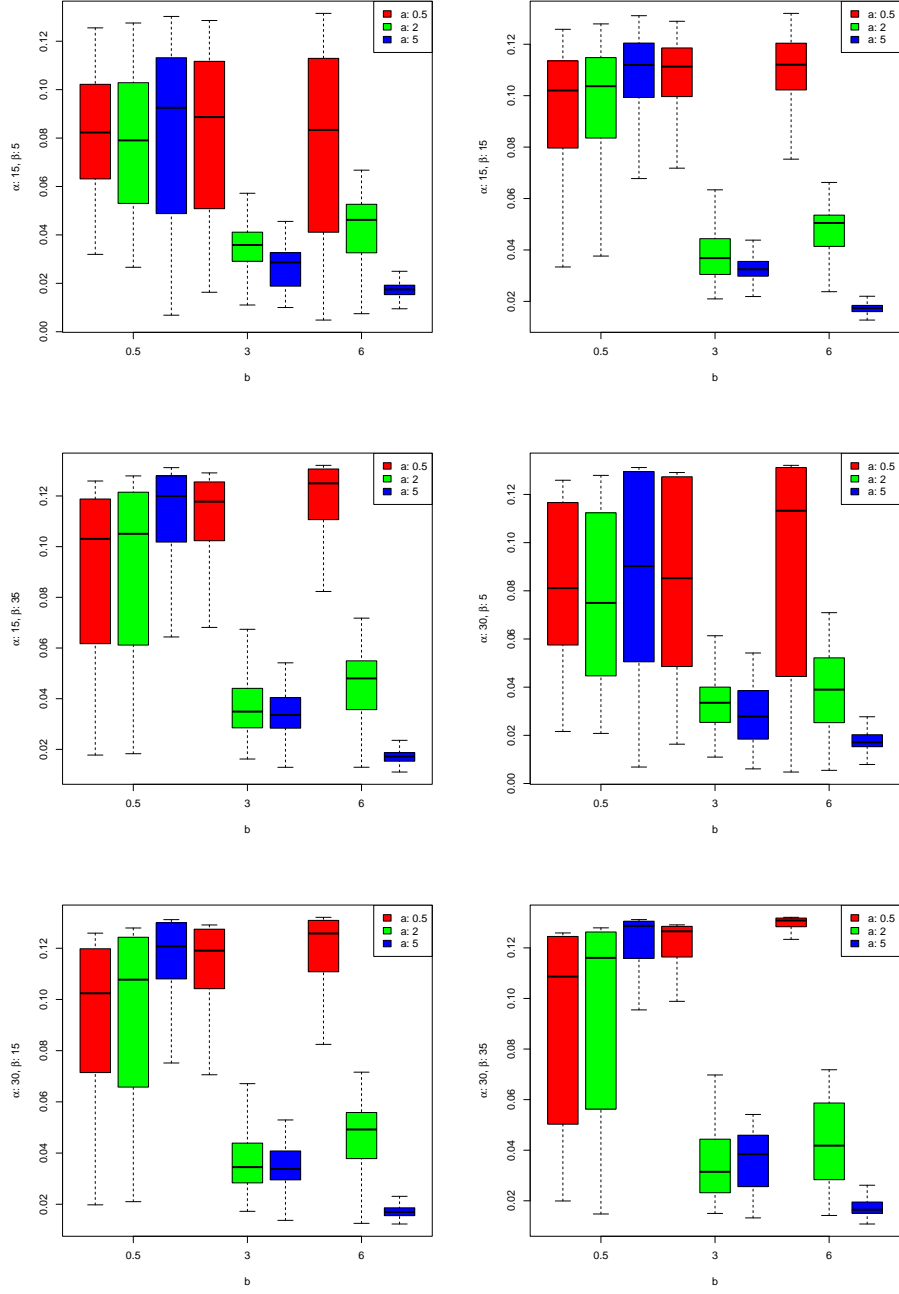

Figure S.7: Boxplots for the estimated Hellinger distance (HD) in the DA analysis for  $\mathcal{K}(a, b)$ .

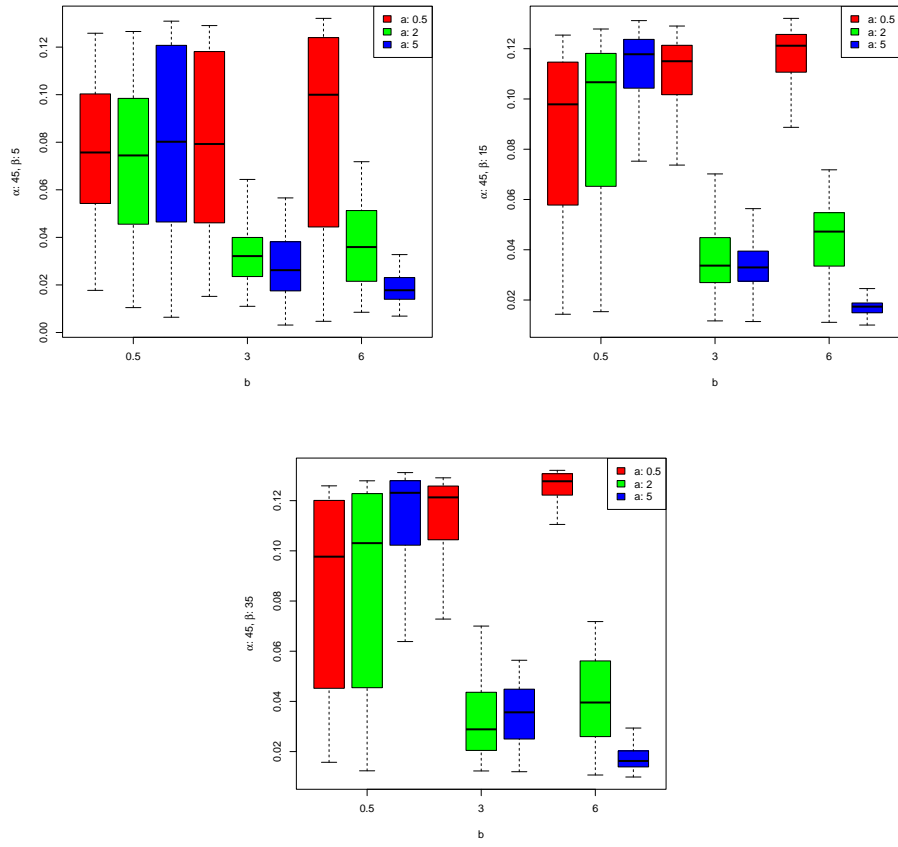

Figure S.8: Boxplots for the estimated Hellinger distance (HD) in the DA analysis for  $\mathcal{K}(a, b)$  (continuation).

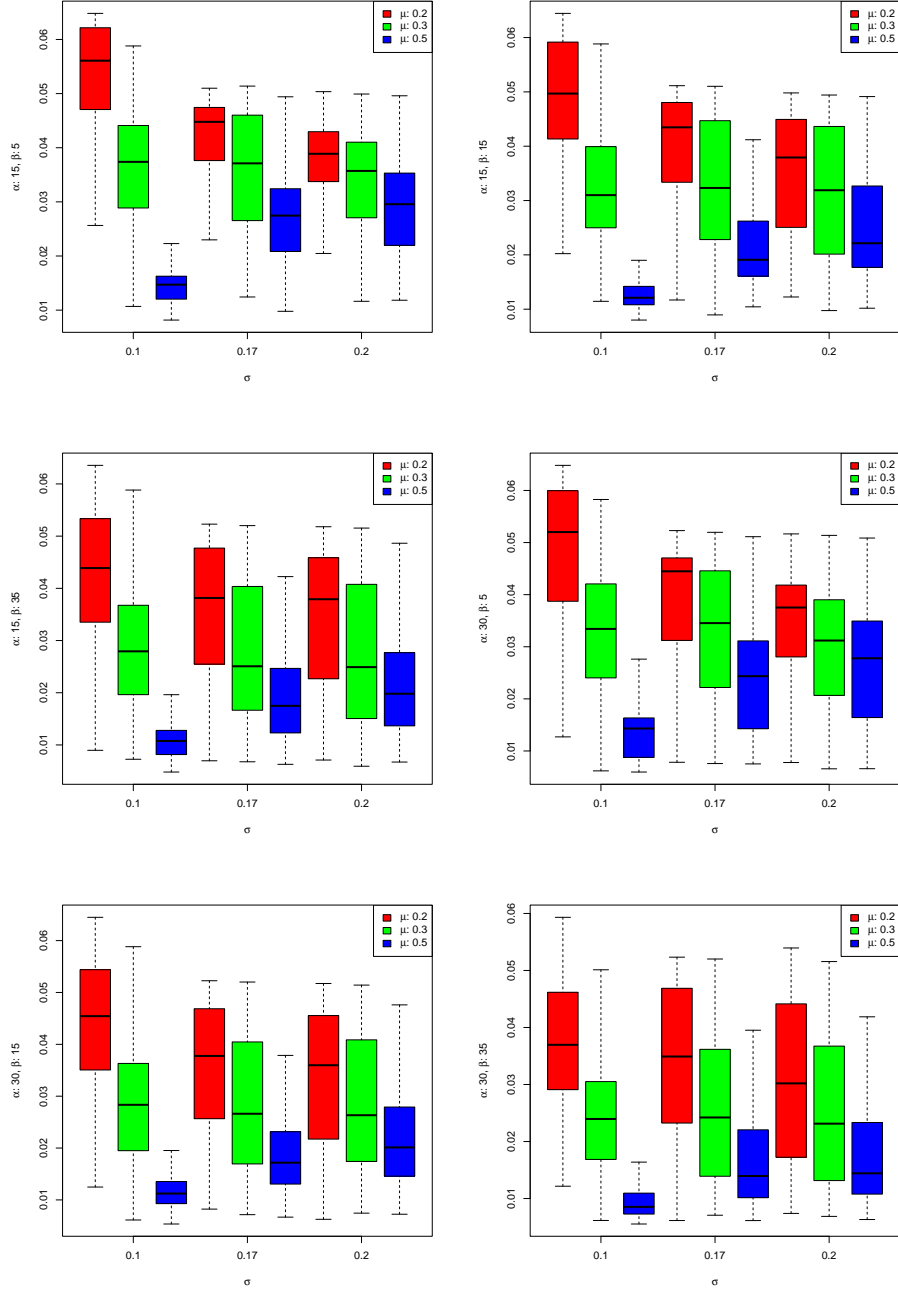

Figure S.9: Boxplots for the estimated total variation (TV) distance in the DA analysis for  $\mathcal{TN}(a, b, \mu, \sigma)$ .

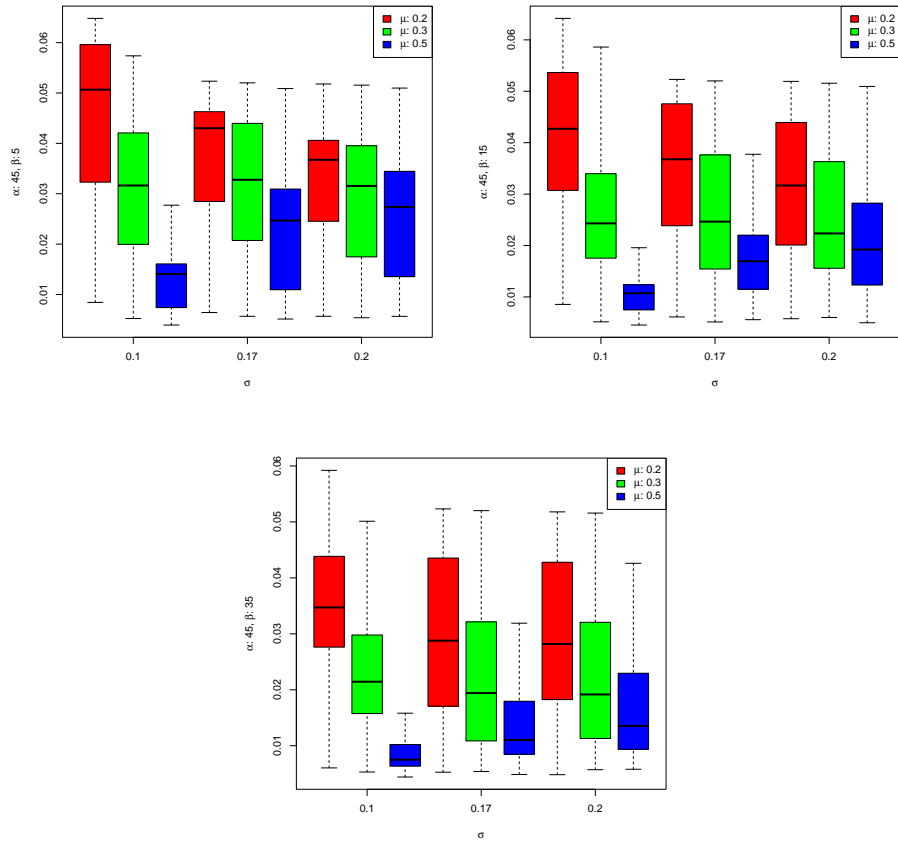

Figure S.10: Boxplots for the estimated total variation (TV) distance in the DA analysis for  $\mathcal{TN}(a, b, \mu, \sigma)$  (continuation).

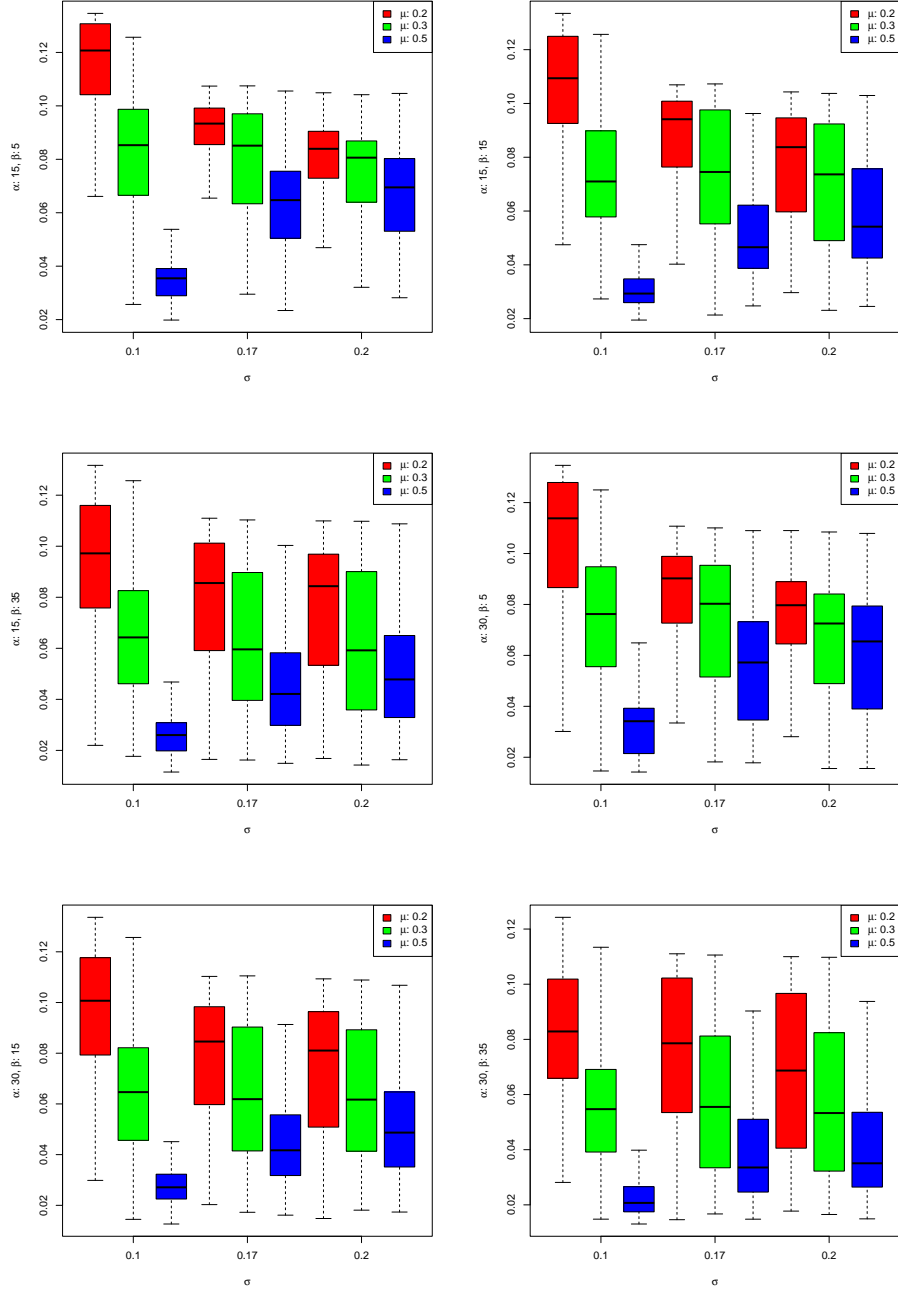

Figure S.11: Boxplots for the estimated Hellinger distance (HD) in the DA analysis for  $\mathcal{TN}(a, b, \mu, \sigma)$ .

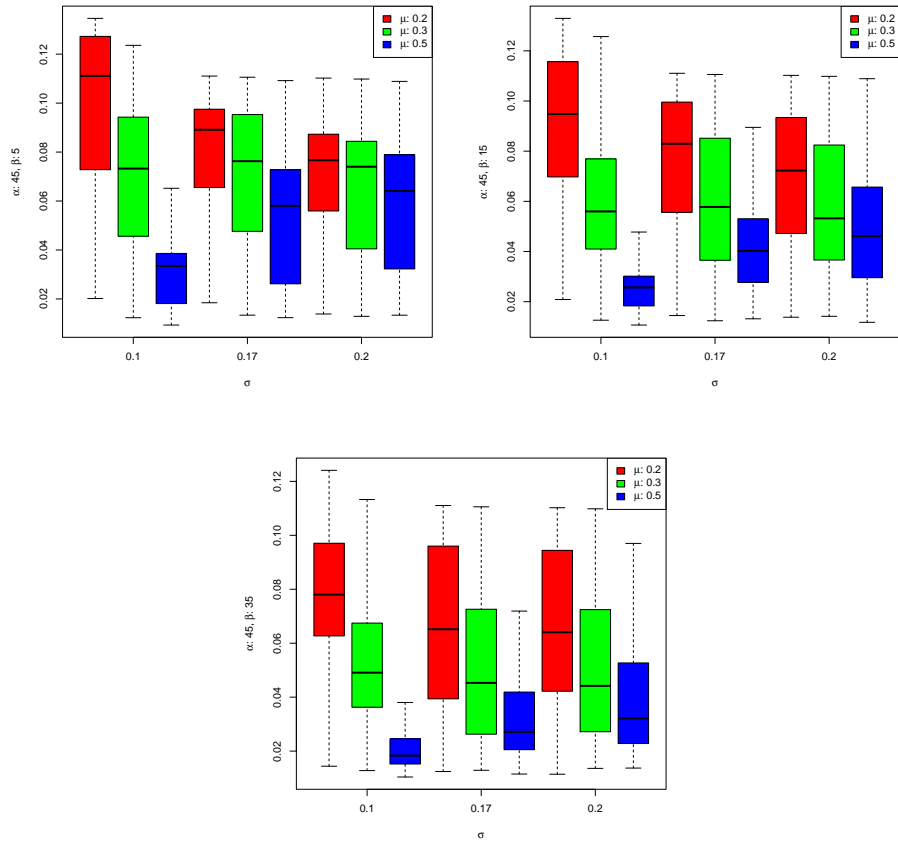

Figure S.12: Boxplots for the estimated Hellinger distance (HD) in the DA analysis for  $\mathcal{TN}(a, b, \mu, \sigma)$  (continuation).

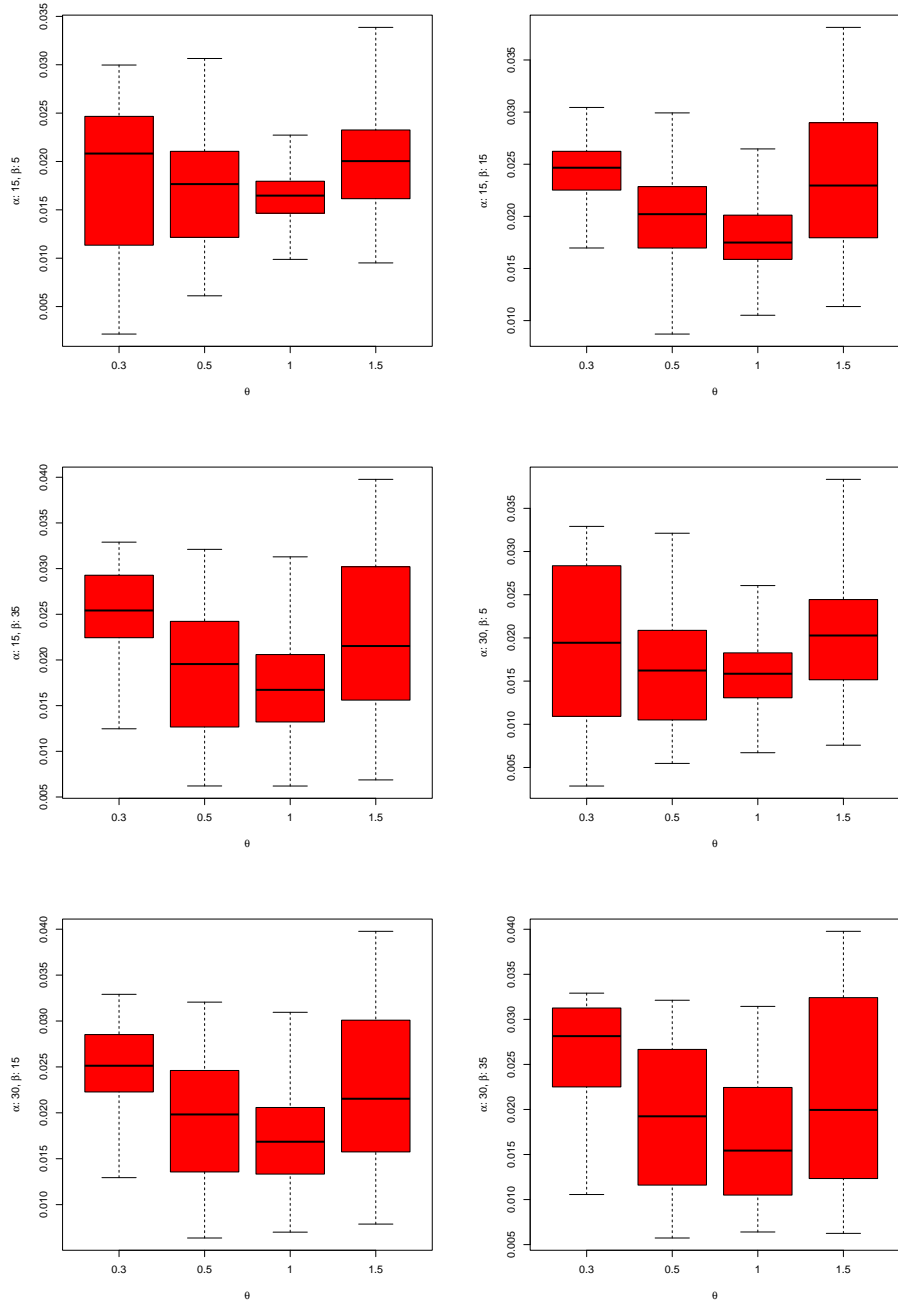

Figure S.13: Boxplots for the estimated total variation (TV) distance in the DA analysis for  $\mathcal{L}\mathcal{B}\mathcal{L}(\theta)$ .

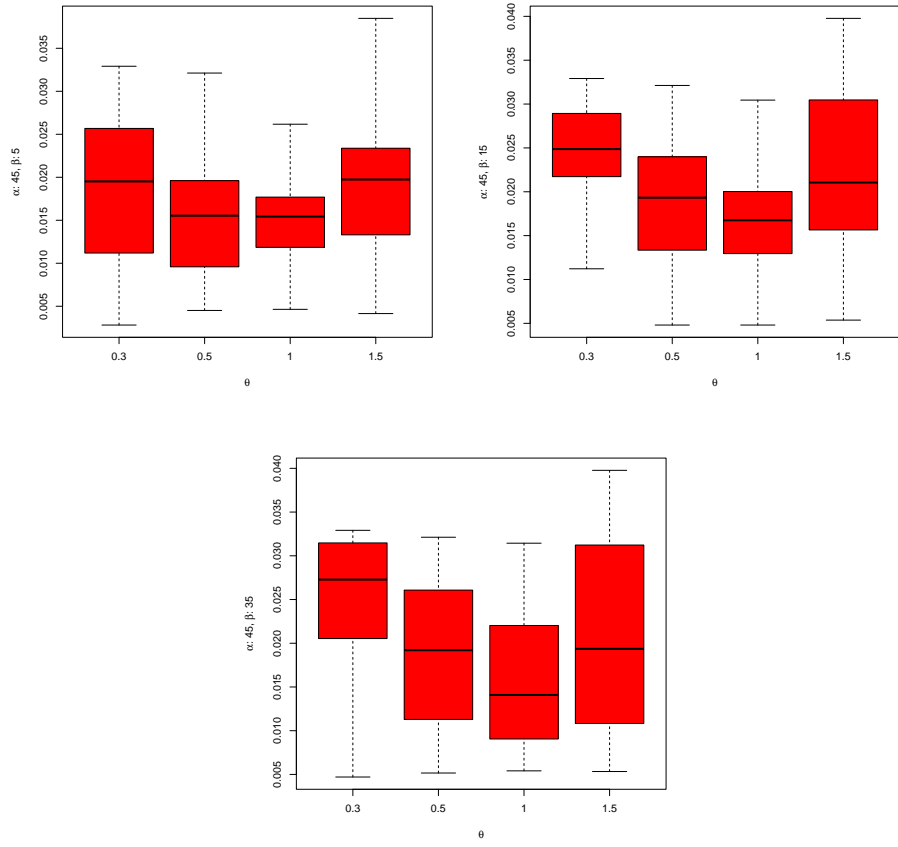

Figure S.14: Boxplots for the estimated total variation (TV) distance in the DA analysis for  $\mathcal{L}\mathcal{B}\mathcal{L}(\theta)$  (continuation).

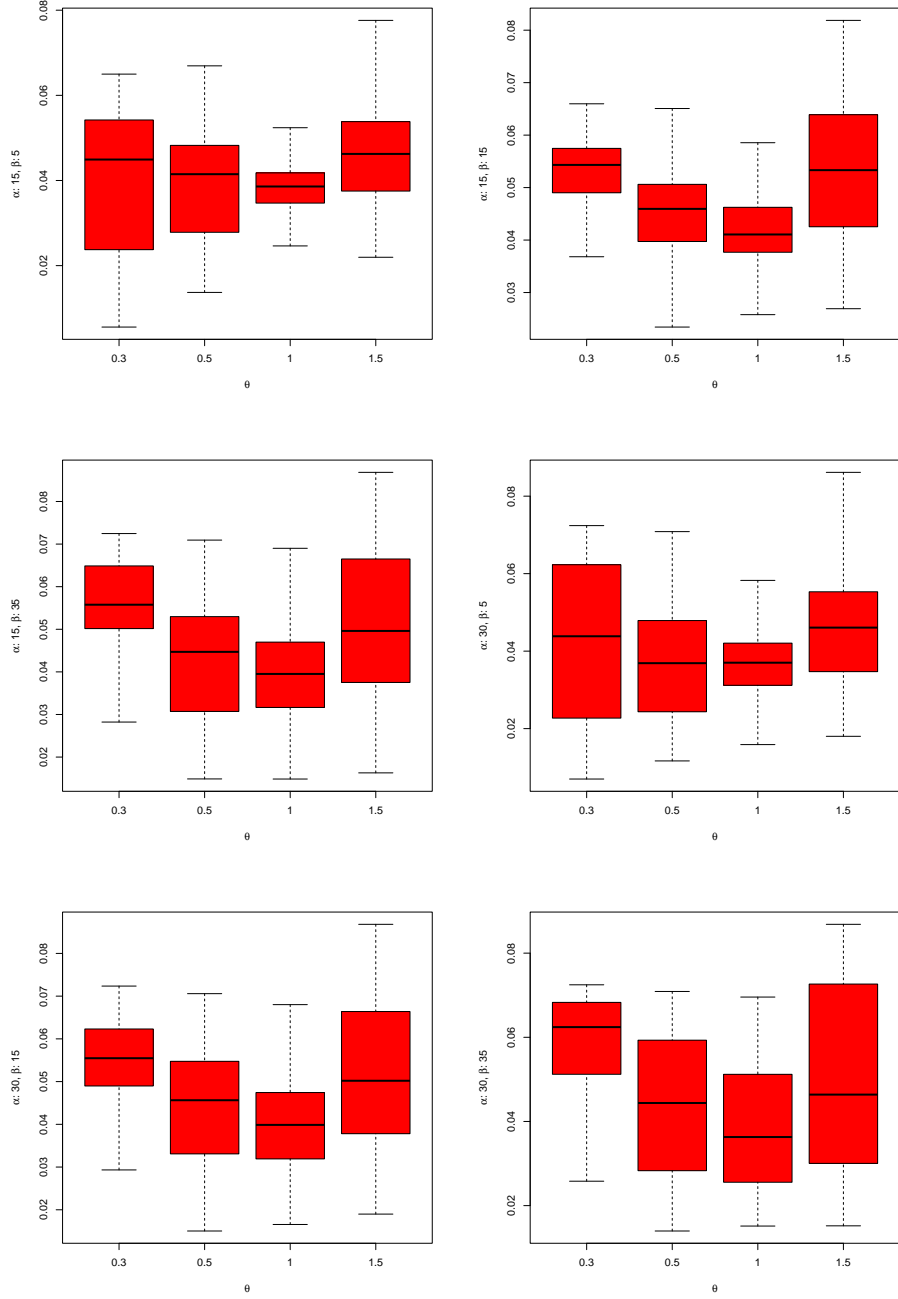

Figure S.15: Boxplots for the estimated Hellinger distance (HD) in the DA analysis for  $\mathcal{L}\mathcal{B}\mathcal{L}(\theta)$ .

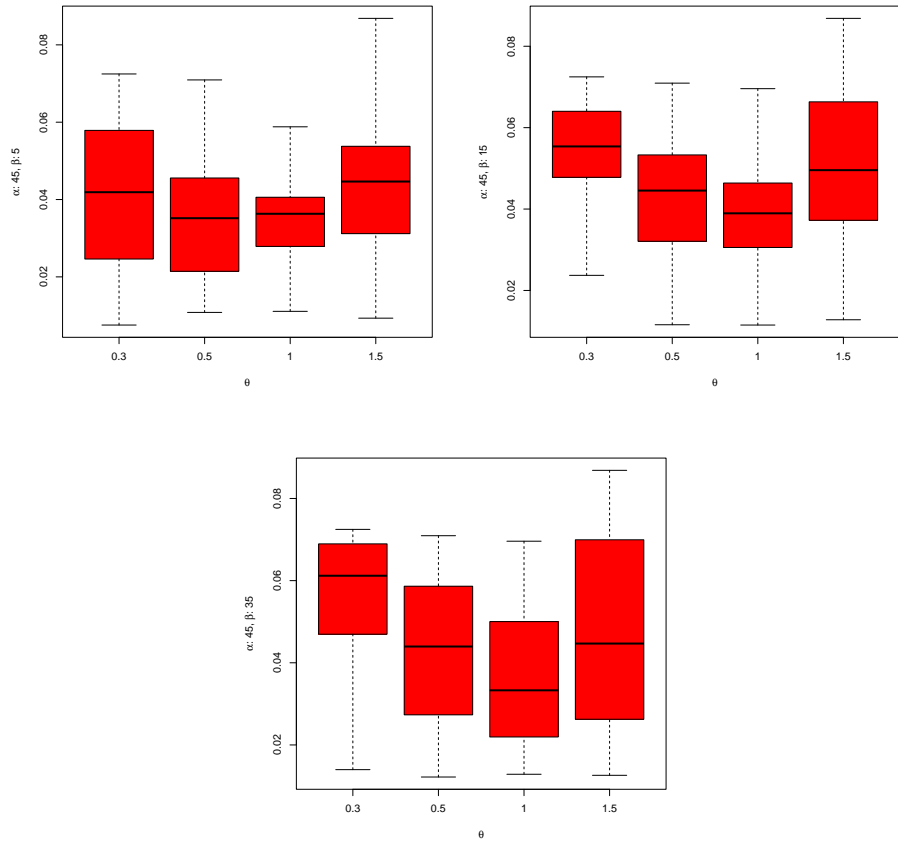

Figure S.16: Boxplots for the estimated Hellinger distance (HD) in the DA analysis for  $\mathcal{L}\mathcal{B}\mathcal{L}(\theta)$  (continuation).

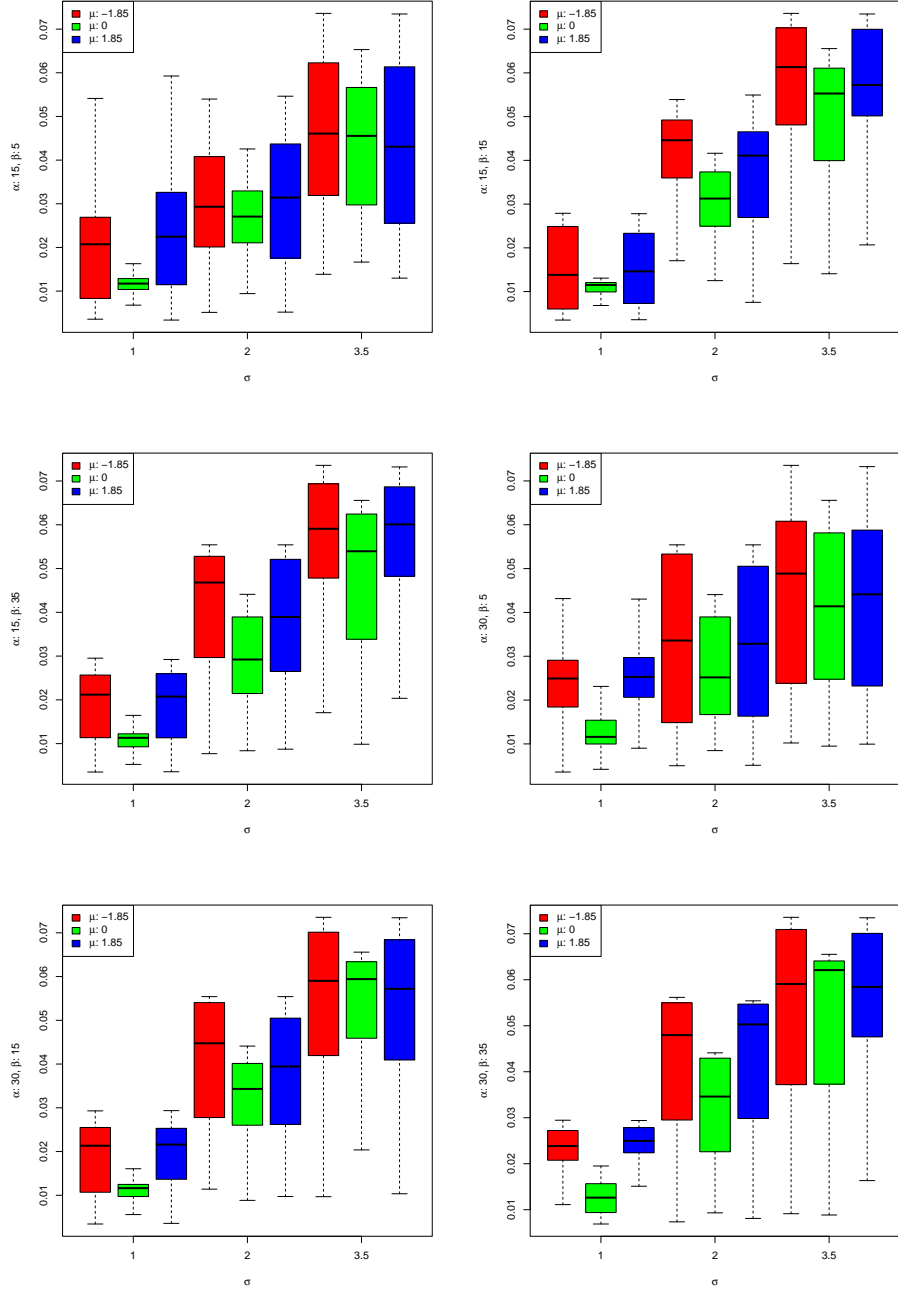

Figure S.17: Boxplots for the estimated total variation (TV) distance in the DA analysis for  $\mathcal{LGN}(\mu, \sigma)$ .

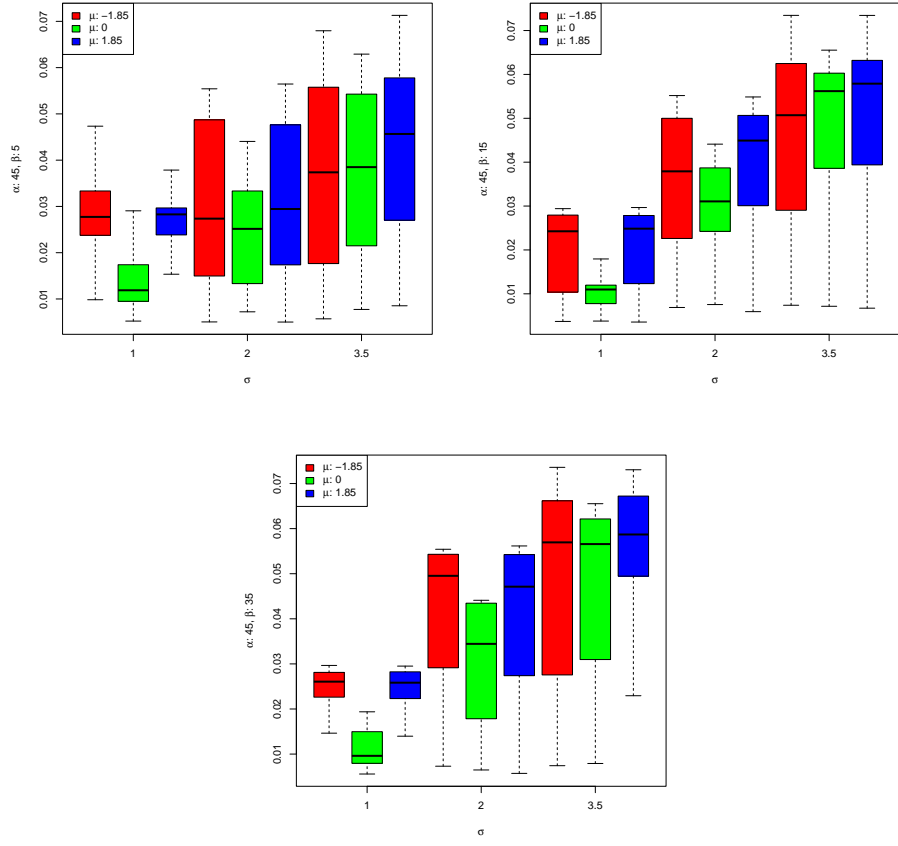

Figure S.18: Boxplots for the estimated total variation (TV) distance in the DA analysis for  $\mathcal{LG}\mathcal{N}(\mu, \sigma)$  (continuation).

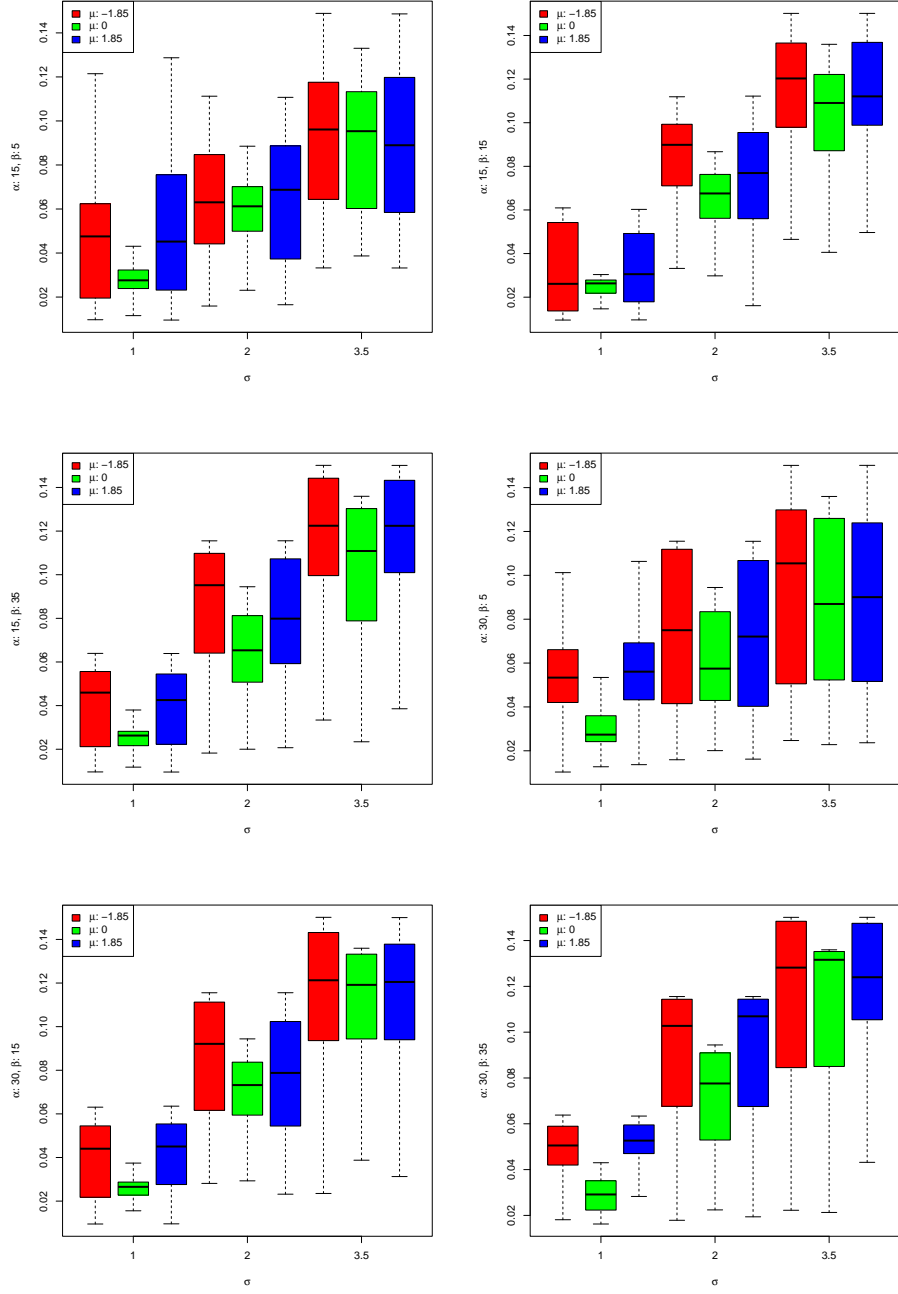

Figure S.19: Boxplots for the estimated Hellinger distance (HD) in the DA analysis for  $\mathcal{LGN}(\mu, \sigma)$ .

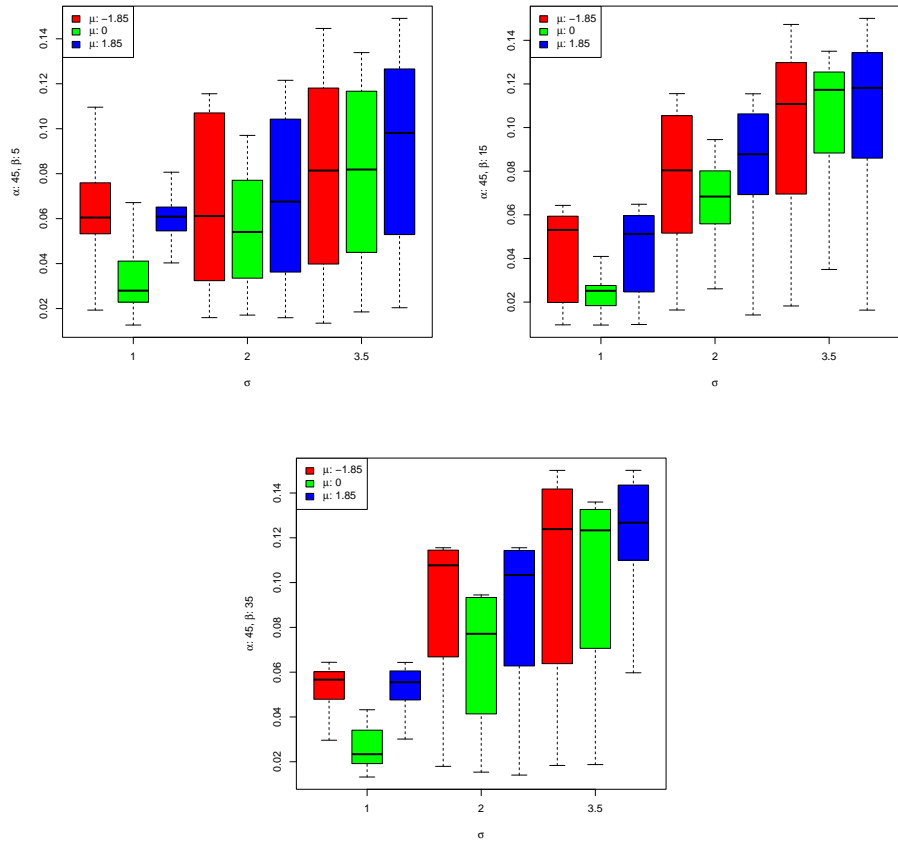

Figure S.20: Boxplots for the estimated Hellinger distance (HD) in the DA analysis for  $\mathcal{LGN}(\mu, \sigma)$  (continuation).
